# Supplementary material for: Safe Reinforcement Learning with Dual Robustness
Source: arXiv:2309.06835 source file (2023-09-13)
Supplement: Supplementary file 1 [file Appendix.tex]

\section*{Appendix}
